# Supplementary material for: InvDiff: Invariant Guidance for Bias Mitigation in Diffusion Models
Source: arXiv:2412.08480 source file (2024-12-11)
Supplement: Supplementary file 2 [file appendix_celeba_sample.tex]

\begin{figure}[!htbp]
    \centering
    \begin{subfigure}[t]{0.4\textwidth}
        \centering
        \includegraphics[width=\textwidth]{Pics/the face of a female celebrity.png}
        \caption{Prompt: the face of a female celebrity}
    \end{subfigure}
    \begin{subfigure}[t]{0.4\textwidth}
        \centering
\includegraphics[width=\textwidth]{Pics/the face of a male celebrity.png}
        \caption{Prompt: the face of a female celebrity}
    \end{subfigure}
    \caption{CelebA results sampled from our model}
    \label{fig:sample_celeba}
    \Description{}
\end{figure}
